# Supplementary material for: First look at the PYTHIA8 hadronization program for neutrino interaction generators
Source: arXiv:1602.00083 source file (2016-01-30)
Supplement: Supplementary file 1 [file jpsj_suppl_template.pdf]

# First Letter of Each Word Should be Capitalized Except for Articles and Conjunctions

Hanako BUTSURI<sup>1</sup> and Taro BUTSURI<sup>2</sup>

<sup>1</sup>*Physical Society of Japan, 5-34-3-5F Shinbashi, Minato, Tokyo 105-0004, Japan*

<sup>2</sup>*JPSJ Editorial Division, Physical Society of Japan, 2-31-22-5F Yushima, Bunkyo, Tokyo 113-0034, Japan*

*E-mail: jpsj\_edit@ipap.jp*

(Received June 23, 2011)

Abstract should state briefly the general aspects of the subject and the main conclusions. It should not contain equations. It is not part of the text and should be complete in itself: no table numbers, figure numbers or references should be given. Keywords below should be chosen as they best describe the contents of the paper. Each keyword, except proper nouns and acronyms, should be typed in lower-case letters and followed by a comma.

**KEYWORDS:** keyword1, keyword2, keyword3, . . .

## 1. Introduction

You can use this file as a template to prepare your manuscript for Supplement to the Journal of the Physical Society of Japan [1, 2].

Copy `jpsj-suppl.cls` and `cite.sty` onto an arbitrary directory under the `texmf` tree, for example, `$texmf/tex/latex/jpsj`. If you have already obtained `cite.sty`, you do not need to copy it.

Many useful commands for equations are available because `jpsj-suppl.cls` automatically loads the `amsmath` package. Please refer to reference books on  $\text{\LaTeX}$  for details on the `amsmath` package.

Please note that we have changed the format of Supplement from two-column layout to one-column. This means that the `twocolumn` option is not available any longer.

## 2. Another Section

### 2.1 Subsection

#### 2.1.1 Subsubsection

**Table I.** Captions to tables and figures should be sentences.

|     |     |
|-----|-----|
| AAA | BBB |
| CCC | DDD |

#### 2.1.2 Equation numbers

The `seceq` option resets the equation numbers at the start of each section.

**Fig. 1.** You can embed figures using the `\includegraphics` command. EPS is the only format that can be embedded. Basically, figures should appear where they are cited in the text. You do not need to separate figures from the main text when you use L<sup>A</sup>T<sub>E</sub>X for preparing your manuscript.

Label figures, tables, and equations appropriately using the `\label` command, and use the `\ref` command to cite them in the text as “as shown in Fig. `\ref{f1}`”. This automatically labels the numbers in numerical order.

The `minipage` environment can be used to place figures horizontally.

$$E = mc^2 \tag{1}$$

## Appendix

Use the `\appendix` command if you need an appendix(es). The `\section` command should follow even though there is no title for the appendix (see above in the source of this file).

## References

- [1] The abbreviation for JPSJ must be “J. Phys. Soc. Jpn.” in the reference list.
- [2] More abbreviations of journal titles are listed in “Instructions for Preparation of Manuscript”, which is available at our Web site (<http://jpsj.ipap.jp>).
- [3] F. Author, S. Author, and T. Author: Abbreviated journal title **volume in bold face** (year of publication) initial page or article ID.
